# Supplementary material for: More than just an auxiliary loss: Anti-spoofing Backbone Training via Adversarial Pseudo-depth Generation
Source: arXiv:2101.00200 source file (2021-03-19)
Supplement: Supplementary file 1 [file 6_Appendix.tex]

\section{Appendix}
\subsection{Implementation Detail}
\label{appendix:Implementation}
% 나은님 여기다가 피규어 넣어주시면 감사하겠습니다.
